# Supplementary material for: The Limitations of Model Uncertainty in Adversarial Settings
Source: arXiv:1812.02606 source file (2019-11-17)
Supplement: Supplementary file 1 [file Appendix.tex]

\section{Detailed Attack Derivation}
In this Appendix we first write the detailed derivation of the JSMA and FGSM attack for GPC, and then describe the training of the surrogates.

\subsection{Derivation of FGSM and JSMA for GP}
In this part of the Appendix, we present the detailed derivation to compute adversarial examples on GPC, including the reasoning why it is sufficient to use the latent mean.

We compute the gradient in the output with respect to the input dimensions. We consider the chain of gradients for the normalized output $ \bar{\sigma_*}= \sigma (f)$, an test  input $x^*$:

\begin{equation}
\frac{\partial \bar{\sigma_*}}{\partial x^*} = \frac{\partial  \bar{\sigma_*}}{\partial f} \times \frac{\partial f}{\partial k} \times \frac{\partial k}{\partial x^*}
\end{equation}
where $f$ is the latent mean and $k$ the covariance function, respectively.

Note that for this attack, we are only interested in the relative order of the gradients, not their actual values. Unfortunately, $\bar{\sigma_*}$ does not vary monotonically with $f$ as the variance also affects the prediction. However, we are in a setting of binary classification, so we are only interested in moving the prediction, $\bar{\sigma_*}$, across the $0.5$ boundary. No change in variance can cause this, instead a change in the mean of $f$ is required (effectively the mean $\bar{\sigma_*}$ is monotonic with respect to $f$ in the region of 0.5). The fastest we can get $\bar{\sigma_*}$ from one probability threshold $p_t$ to its opposite $1-p_t$ is when there is no variance (any variance will move the mean $\bar{\sigma_*}$ towards 0.5). So finding the gradient of $f$ is sufficient. This is analogous to the usage of the logits (instead of the softmax) in evasion attacks on deep neural networks.

However, we found that we can still use the gradient of $f$ (instead of a numerical approximation to $ \bar{\sigma_*}$):

\begin{equation}
\label{eq:derivA}
\frac{\partial f}{\partial x^*} = \frac{\partial  f}{\partial k} \times \frac{\partial k}{\partial x^*}
\end{equation}

Let us first rewrite the expected value of $f$ given a single test point $x^*$: 

\begin{equation}
E[f_*] = K^{*T} K^{-1}Y_{GP}
\end{equation}
Where we write $Y_{GP}$ to denote GPC's output for the training points $X$. Hence, $f(X)=Y_{GP}$
 From here, we move on to the first part of the gradient,
\begin{equation}
\label{eq:fstargradA}
\frac{\partial f}{\partial k} = K^{-1}Y_{GP}
\end{equation}
note the remaining terms are both constant with respect to the test input $x^*$. The gradient of the covariance with respect to the inputs depends on the particular kernel that is applied. In our case, for the RBF kernel, between training point $x \in X_{tr}$ and test point $x^*$, the gradient can be expressed as
\begin{equation}
\label{eq:kerngradA}
\frac{\partial k(x^*,x)}{\partial x^*_{i}} = \frac{1}{l^2} (x_{i} - x^*_{i}) k(x^*,x)
\end{equation}
where $x_i$ and $x^*_i$ each denote feature or dimension $i$ of the corresponding vector or data point and $l$ denotes the length-scale parameter of the kernel. Using \cref{eq:derivA} the gradient of the output $\bar{\sigma_*}$ with respect to the inputs is approximately proportional to the product of \cref{eq:fstargradA} and \cref{eq:kerngradA}, in the region of $0.5$.

Based on the computation of these gradients, we perturb the initial sample. In GPFGS (%\cref{alg::GPFGS}, 
similar to FGSM), we introduce a global change using the sign of the gradient and a specified $\epsilon$. 

Alternatively in GPJM, we compute local, greedy changes (see \cref{alg::GPJM}, 
analogous to JSMA). Instead of a saliency map, however, we iteratively compute the (still unperturbed) feature with the strongest gradient and perturb it. We alternate between perturbation for misclassification and (optionally) decreasing uncertainty. We finish altering the example when it is either misclassified at a predefined threshold, or in case we have changed more than a previously specified number of features, corresponding to a fail. 

\begin{algorithm}
\caption{GPFGS}\label{alg::GPFGS}
\begin{algorithmic}[1]
\State {\bfseries Input:} sample $\mathbf{x}$, latent function $f_*$, parameter $\mathbf{\epsilon}$
\State $\mathbf{x^*}\leftarrow \mathbf{x} + \epsilon \times $sign$(\nabla f_* )$ \\
\Return $\mathbf{x^*}$
\end{algorithmic}
\end{algorithm}

\begin{algorithm}[!t]
\caption{GPJM}
\label{alg::GPJM}
\begin{algorithmic}[1]
\State {\bfseries Input:} sample $\mathbf{x}_{adv}=\mathbf{x^{*}}$, latent function $f^*$, classifier $\bar{\sigma_*}$, threshold $t$, threshold varT, desired confidence $c$, changed=$[]$,
\Repeat
    \If{len$($changed$)>t$} \Return fail \EndIf
	\State grads$_m$ $\leftarrow \nabla $mean$(f^*(\mathbf{x}_{adv})) $ \emph{\#  classification}
	\State changed,$\mathbf{x}_{adv}, \leftarrow$ perturb($\mathbf{x}_{adv},$grads$_m,$changed$)$
	\Repeat
	    \If{len$($changed$)>t$} \Return fail \EndIf
		\State grads$_v$ $\leftarrow \nabla $var$(f^*(\mathbf{x}_{adv})) $ \emph{\#  uncertainty}
	    \State changed,$\mathbf{x}_{adv}, \leftarrow$ perturb($\mathbf{x}_{adv},$grads$_v,$changed$)$
    \Until{var$f^*(\mathbf{x}_{adv})) \leq$ varT}
\Until{classified$(\bar{\sigma_*(\mathbf{x}_{adv})}),c)$} \\
\Return $\mathbf{x}_{adv}$
\end{algorithmic}
\end{algorithm}

\subsection{Surrogates Models for GP}
We train several surrogate models to approximate GP's decision surface and to be able to apply DNN specific attack to GPC as well. To this end, we first briefly introduce Gaussian process latent variable model (GPLVM) these surrogates are trained with, before we introduce the attacks themselves. 

\begin{figure}[t]
\centering
\includegraphics[width=.99\linewidth]{LSAN.pdf}
\caption{The intuition approximating the latent using DNN. The first network is trained on a latent space, the second to classify input from this latent space. After training, the two networks are combined and yield one DNN classifier. }\label{fig:latent2net}
\end{figure}

\subsubsection{GP Latent Variable Model} 
GPC learns based on labeled data. This introduces an implicit bias: we assume for example that the number of labels is finite and fixed, and that the labels are related to the structure of the data.
%first problem
Furthermore, the curse of dimensionality affects classification. This curse affects distance measure on data points. In higher dimensions, the ratio between nearest and furthest point approximates one. All data points are thus uniformly distant, impeding classification: it becomes harder to compute a separating boundary. Consequently, we are interested in finding a lower dimensional representation of our data.
%second problem

These two issues are taken into account when using the Gaussian process latent variable model (GPLVM). Analogously to GPC, GPLVM models uncertainty estimates. Further, its latent space allows for nonlinear connections in the feature space to be represented. Yet, this latent space or lower-dimensional representation ignores labels. Consequently, we need to apply a classifier on top of GPLVM to enable classification.

\subsubsection{Training Surrogates.}
We propose a complementary approach to the attacks on GPC by attacking GPLVM+SVM using (the already established methodology of) DNN surrogates specifically tailored for the GP. To train such a surrogate model, we train a DNN to fit the latent space representation of GPLVM in one of the hidden layers. 
We achieve this by taking a common DNN and splitting it into two parts, where a hidden layer becomes the output layer for the first part and the input layer for the second part (see lower half of \cref{fig:latent2net}). 

The training data is fed as input to the first part. 
We train it minimizing the loss between the output of the network and the latent space we want to approximate (for example the output of GPLVM). 
The second part receives this latent space as input, and is trained minimizing the loss to the normal labels. 
When stacking these two networks (i.e., when feeding the output of the first part immediately into the second), we obtain a combined DNN that mimics both the latent space it was trained on and the classifier on this latent space.
